# Supplementary material for: Emergent B2 chemical orderings in the AlTiVNb and AlTiCrMo refractory high-entropy superalloys studied via first-principles theory and atomistic modelling
Source: arXiv:2503.13235 ancillary file (2025-03-17)
Supplement: Supplementary file 1 [file supplementary_material.pdf]

# Emergent B2 chemical orderings in the AlTiVNb and AlTiCrMo refractory high-entropy superalloys studied via first principles theory and atomistic simulations
# Supplementary Material

Christopher D. Woodgate,[1,*] Hubert J. Naguszewski,[2] David Redka,[3,4] Ján Minár,[4] David Quigley,[2] and Julie B. Staunton[2]

[1]*H.H. Wills Physics Laboratory, University of Bristol, Royal Fort, Bristol, BS8 1TL, United Kingdom*
[2]*Department of Physics, University of Warwick, Coventry, CV4 7AL, United Kingdom*
[3]*Department of Applied Sciences and Mechatronics, Munich University of Applied Sciences HM, Munich, Germany*
[4]*New Technologies Research Center, University of West Bohemia, Pilsen, Czech Republic*

This is the supplementary material accompanying the main text. Here we give values of partial lattice site occupancies as a function of B2 atomic order parameter, show plots of the site/species/orbital-resolved electronic density of states for the predicted B2 chemically ordered structures, tabulate our fitted atom-atom effective pair interactions, and provide an in-depth discussion of the electronic mechanism resulting in an increased residual resistivity for the B2 ordered structures as compared to the A2 phase.

## I. PARTIAL LATTICE SITE OCCUPANCIES AS A FUNCTION OF ATOMIC ORDER PARAMETER

Tables I and II give partial lattice site occupancies for the AlTiVNb and AlTiCrMo as a function of atomic order parameter, $\eta$, for the B2 orderings predicted via our concentration wave analysis.

## II. SITE-RESOLVED ELECTRONIC DENSITY OF STATES

Figs. 1 and 2 show the site-projected total electronic density of states (DoS) smoothly varying for increasing order parameter $\eta$ for AlTiVNb and AlTiCrMo. The gradual transition from disordered to ordered state is clearly visible for both alloys, especially the development of the additional peak at the 1b position of AlTiVNb by about 1 eV. Note that in this representation, the contributions from separate atoms on each of the 1a and 1b lattice sites are weighted by their respective concentrations to give the total EDoS.

## III. ATOM-ATOM EFFECTIVE PAIR INTERACTIONS

Tables III and IV give our atom-atom effective pair interactions recovered from the *ab initio* data, fitted to the first six coordination shells of the bcc lattice. The atom-atom effective pair interactions are for the Bragg-Williams Hamiltonian, which takes the form

$$H = \frac{1}{2} \sum_{i\alpha;j\alpha'} V_{i\alpha;j\alpha'} \xi_{i\alpha} \xi_{j\alpha'}. \tag{1}$$

However, assuming interactions are isotropic, we can write $V^{(n)}_{\alpha\alpha'}$ to denote the interaction between species $\alpha$ and $\alpha'$ on coordination shell $n$. Then Eq. 1 takes the form

$$H = \frac{1}{2} \sum_i \sum_n \left( \sum_{j \in n(i)} \sum_{\alpha\alpha'} V^{(n)}_{\alpha\alpha'} \xi_{i\alpha} \xi_{j\alpha'} \right), \tag{2}$$

where $n(i)$ denotes the set of lattice sites which are $n$th nearest-neighbours to site $i$.

* christopher.woodgate@bristol.ac.uk

| $\eta$ | 1a Site Partial Occupancies | | | | 1b Site Partial Occupancies | | | |
|---|---|---|---|---|---|---|---|---|
| | Al | Ti | V | Nb | Al | Ti | V | Nb |
| 0.0 | 0.250 | 0.250 | 0.250 | 0.250 | 0.250 | 0.250 | 0.250 | 0.250 |
| 0.1 | 0.275 | 0.230 | 0.237 | 0.258 | 0.225 | 0.270 | 0.263 | 0.242 |
| 0.2 | 0.300 | 0.209 | 0.224 | 0.267 | 0.200 | 0.291 | 0.276 | 0.233 |
| 0.3 | 0.325 | 0.189 | 0.211 | 0.275 | 0.175 | 0.311 | 0.289 | 0.225 |
| 0.4 | 0.350 | 0.168 | 0.198 | 0.283 | 0.150 | 0.332 | 0.302 | 0.217 |
| 0.5 | 0.375 | 0.148 | 0.186 | 0.291 | 0.125 | 0.352 | 0.314 | 0.209 |
| 0.6 | 0.400 | 0.128 | 0.173 | 0.300 | 0.100 | 0.372 | 0.327 | 0.200 |
| 0.7 | 0.425 | 0.107 | 0.160 | 0.308 | 0.075 | 0.393 | 0.340 | 0.192 |
| 0.8 | 0.450 | 0.087 | 0.147 | 0.316 | 0.050 | 0.413 | 0.353 | 0.184 |
| 0.9 | 0.475 | 0.067 | 0.134 | 0.324 | 0.025 | 0.433 | 0.366 | 0.176 |
| 1.0 | 0.500 | 0.046 | 0.121 | 0.333 | 0.000 | 0.454 | 0.379 | 0.167 |

TABLE I. Partial lattice site occupancies for the B2 chemical ordering predicted by our concentration wave analysis for the AlTiVNb RSA as a function of atomic long-range order parameter, $\eta$. The two non-equivalent lattice sites in the B2 (CsCl) structure are given their Wyckoff labels. The case $\eta = 0$ corresponds to the disordered bcc (A2) solid solution. The case $\eta = 1$ corresponds to largest chemical fluctuation consistent with the polarisation of our predicted concentration wave.

| $\eta$ | 1a Site Partial Occupancies | | | | 1b Site Partial Occupancies | | | |
|---|---|---|---|---|---|---|---|---|
| | Al | Ti | Cr | Mo | Al | Ti | Cr | Mo |
| 0.0 | 0.250 | 0.250 | 0.250 | 0.250 | 0.250 | 0.250 | 0.250 | 0.250 |
| 0.1 | 0.234 | 0.275 | 0.251 | 0.240 | 0.266 | 0.225 | 0.249 | 0.260 |
| 0.2 | 0.217 | 0.300 | 0.253 | 0.230 | 0.283 | 0.200 | 0.247 | 0.270 |
| 0.3 | 0.201 | 0.325 | 0.254 | 0.220 | 0.299 | 0.175 | 0.246 | 0.280 |
| 0.4 | 0.184 | 0.350 | 0.256 | 0.210 | 0.316 | 0.150 | 0.244 | 0.290 |
| 0.5 | 0.168 | 0.375 | 0.257 | 0.200 | 0.332 | 0.125 | 0.243 | 0.300 |
| 0.6 | 0.151 | 0.400 | 0.258 | 0.190 | 0.349 | 0.100 | 0.242 | 0.310 |
| 0.7 | 0.135 | 0.425 | 0.260 | 0.180 | 0.365 | 0.075 | 0.240 | 0.320 |
| 0.8 | 0.118 | 0.450 | 0.261 | 0.170 | 0.382 | 0.050 | 0.239 | 0.330 |
| 0.9 | 0.102 | 0.475 | 0.263 | 0.161 | 0.398 | 0.025 | 0.237 | 0.339 |
| 1.0 | 0.085 | 0.500 | 0.264 | 0.151 | 0.415 | 0.000 | 0.236 | 0.349 |

TABLE II. Partial lattice site occupancies for the B2 chemical ordering predicted by our concentration wave analysis for the AlTiCrMo RSA as a function of atomic long-range order parameter, $\eta$. The two non-equivalent lattice sites in the B2 (CsCl) structure are given their Wyckoff labels. The case $\eta = 0$ corresponds to the disordered bcc (A2) solid solution. The case $\eta = 1$ corresponds to largest chemical fluctuation consistent with the polarisation of our predicted concentration wave.

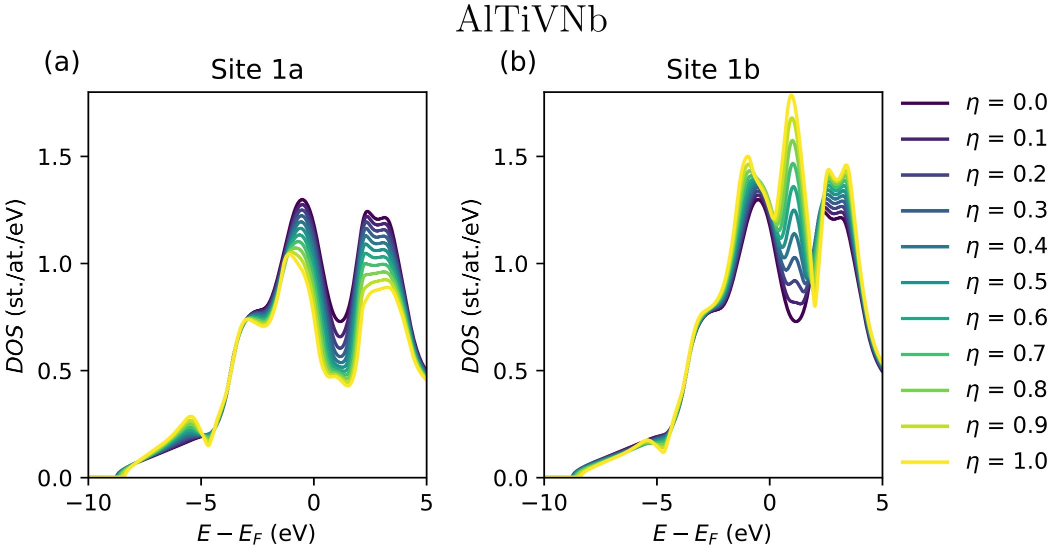


FIG. 1. Comparison of the electronic density of states (DoS) for the AlTiVNb RSA within inreasing order parameter $\eta$ resolved into its separate contributions from the 1a and 1b positions of the B2 ordered structure.

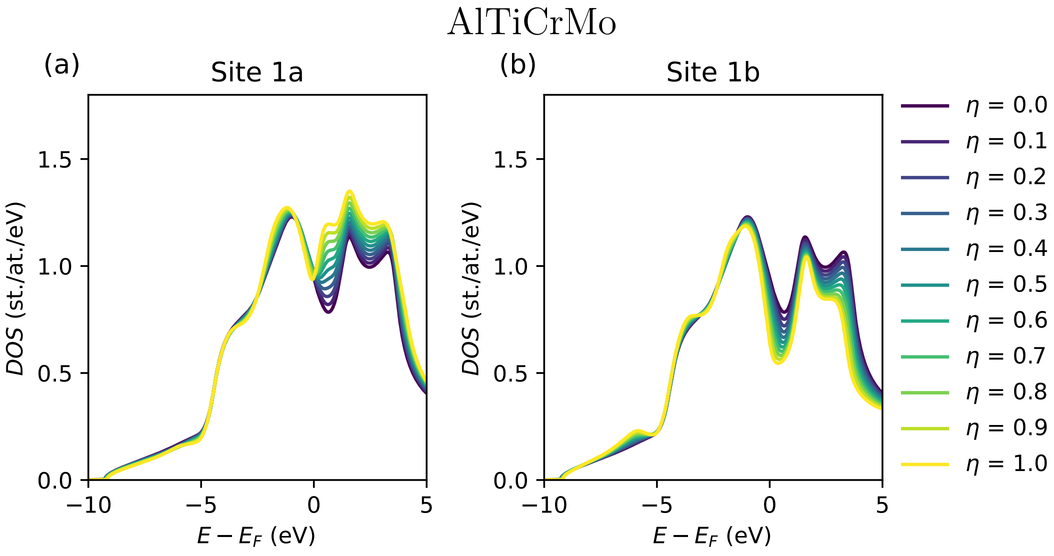


FIG. 2. Comparison of the electronic density of states (DoS) for the AlTiCrMo RSA within inreasing order parameter $\eta$ resolved into its separate contributions from the 1a and 1b positions of the B2 ordered structure.

| $V^{(1)}_{\alpha\alpha'}$ | Al | Ti | V | Nb | $V^{(2)}_{\alpha\alpha'}$ | Al | Ti | V | Nb |
|---|---|---|---|---|---|---|---|---|---|
| Al | 6.8 | −50.3 | −18.7 | 62.2 | Al | −2.7 | 14.7 | 17.6 | −29.6 |
| Ti | −50.3 | 31.0 | 12.8 | 6.6 | Ti | 14.7 | 2.7 | −5.0 | −12.5 |
| V | −18.7 | 12.8 | 15.5 | −9.5 | V | 17.6 | −5.0 | 0.0 | −12.6 |
| Nb | 62.2 | 6.6 | −9.5 | −59.2 | Nb | −29.6 | −12.5 | −12.6 | 54.7 |
| $V^{(3)}_{\alpha\alpha'}$ | Al | Ti | V | Nb | $V^{(4)}_{\alpha\alpha'}$ | Al | Ti | V | Nb |
| Al | 24.4 | −7.6 | −2.4 | −14.4 | Al | 10.5 | −5.4 | −4.3 | −0.8 |
| Ti | −7.6 | 2.3 | 2.3 | 3.0 | Ti | −5.4 | 1.5 | 1.6 | 2.3 |
| V | −2.4 | 2.3 | 1.9 | −1.8 | V | −4.3 | 1.6 | −0.2 | 3.0 |
| Nb | −14.4 | 3.0 | −1.8 | 13.1 | Nb | −0.8 | 2.3 | 3.0 | −4.4 |
| $V^{(5)}_{\alpha\alpha'}$ | Al | Ti | V | Nb | $V^{(6)}_{\alpha\alpha'}$ | Al | Ti | V | Nb |
| Al | −6.0 | 4.3 | 3.9 | −2.2 | Al | −2.6 | 1.6 | 0.5 | 0.6 |
| Ti | 4.3 | −1.5 | −1.1 | −1.7 | Ti | 1.6 | −0.1 | −0.2 | −1.3 |
| V | 3.9 | −1.1 | −1.1 | −1.8 | V | 0.5 | −0.2 | 0.2 | −0.5 |
| Nb | −2.2 | −1.7 | −1.8 | 5.6 | Nb | 0.6 | −1.3 | −0.5 | 1.1 |

TABLE III. Fitted atom-atom effective pair interactions for the AlTiVNb RSA. The interaction is fitted to the first six coordination shells of the bcc lattice. All energies in units of meV.

| $V^{(1)}_{\alpha\alpha'}$ | Al | Ti | Cr | Mo | $V^{(2)}_{\alpha\alpha'}$ | Al | Ti | Cr | Mo |
|---|---|---|---|---|---|---|---|---|---|
| Al | −9.9 | −32.6 | −7.2 | 49.6 | Al | 21.0 | 5.0 | 3.1 | −29.0 |
| Ti | −32.6 | 70.1 | −10.0 | −27.5 | Ti | 5.0 | 17.5 | −6.9 | −15.6 |
| Cr | −7.2 | −10.0 | 16.0 | 1.1 | Cr | 3.1 | −6.9 | 13.7 | −9.8 |
| Mo | 49.6 | −27.5 | 1.1 | −23.2 | Mo | −29.0 | −15.6 | −9.8 | 54.4 |
| $V^{(3)}_{\alpha\alpha'}$ | Al | Ti | Cr | Mo | $V^{(4)}_{\alpha\alpha'}$ | Al | Ti | Cr | Mo |
| Al | 14.9 | −8.3 | 1.9 | −8.5 | Al | −1.5 | −7.3 | 1.5 | 7.2 |
| Ti | −8.3 | 6.0 | 0.3 | 2.0 | Ti | −7.3 | 4.5 | 1.9 | 0.9 |
| Cr | 1.9 | 0.3 | −0.5 | −1.7 | Cr | 1.5 | 1.9 | −2.8 | −0.6 |
| Mo | −8.5 | 2.0 | −1.7 | 8.3 | Mo | 7.2 | 0.9 | −0.6 | −7.5 |
| $V^{(5)}_{\alpha\alpha'}$ | Al | Ti | Cr | Mo | $V^{(6)}_{\alpha\alpha'}$ | Al | Ti | Cr | Mo |
| Al | −3.1 | 6.4 | 1.6 | −4.8 | Al | 6.0 | −0.2 | −2.4 | −3.4 |
| Ti | 6.4 | −2.8 | −1.3 | −2.2 | Ti | −0.2 | −0.2 | 0.3 | 0.1 |
| Cr | 1.6 | −1.3 | −0.7 | 0.4 | Cr | −2.4 | 0.3 | 0.6 | 1.5 |
| Mo | −4.8 | −2.2 | 0.4 | 6.7 | Mo | −3.4 | 0.1 | 1.5 | 1.7 |

TABLE IV. Fitted atom-atom effective pair interactions for the AlTiCrMo RSA. The interaction is fitted to the first six coordination shells of the bcc lattice. All energies in units of meV.

## IV. SEMI-CLASSICAL APPROACH TO RESIDUAL RESISTIVITY AND DOS ANALYSIS

The Kubo formalism, employed in the main manuscript to compute the residual resistivity, yields only a number (or the diagonal components of the conductivity tensor in our case). Consequently, the physical interpretation of the increase in residual resistivity with increasing order parameter $\eta$ remains somewhat limited. To provide additional insight, we adopt a semi-classical approach based on the Boltzmann transport equation (BTE) within the relaxation time approximation [1]. In this framework, the electrical conductivity tensor $\sigma_{ij}$ is given by [2, 3]

$$\sigma_{ij} = \int_{\mathrm{BZ}} \mathrm{d}E \left(-\frac{\partial f}{\partial E}\right) X_{ij}(E), \tag{3}$$

where $f$ is the Fermi-Dirac distribution, and the transport distribution function is defined as

$$X_{ij}(E) = e^2 \int_{\mathrm{BZ}} \frac{\mathrm{d}\mathbf{k}}{(2\pi)^3} \delta(E - E_{\mathbf{k}}) v_{\mathbf{k},i} v_{\mathbf{k},j} \tau_{\mathbf{k}}. \tag{4}$$

Here, $e$ denotes the elementary charge, $\mathbf{k}$ the wavevector, and $E_{\mathbf{k}}$ the electronic dispersion. The group velocity component in the $i$-th direction is given by $v_{\mathbf{k},i} = \frac{1}{\hbar}\frac{\partial E_{\mathbf{k}}}{\partial k_i}$, while $\tau_{\mathbf{k}}$ represents the $\mathbf{k}$-dependent relaxation time. The integration extends over the entire first Brillouin zone (BZ).

At zero temperature ($T = 0$ K), the conductivity simplifies to $\sigma_{ij} = X_{ij}(E_F)$, where $E_F$ is the Fermi energy. To facilitate the evaluation of $X_{ij}(E_F)$, we introduce an energy-dependent average over possible wavevectors,

$$\langle A_{\mathbf{k},ij} \rangle_E = \frac{\int \frac{\mathrm{d}\mathbf{k}}{(2\pi)^3} \delta(E - E_{\mathbf{k}}) A_{\mathbf{k}}}{g(E)}, \tag{5}$$

where the electronic density of states (DOS) is defined as

$$g(E) = \int_{\mathrm{BZ}} \frac{\mathrm{d}\mathbf{k}}{(2\pi)^3} \delta(E - E_{\mathbf{k}}). \tag{6}$$

For $A_{\mathbf{k},ij} = v_{\mathbf{k},i} v_{\mathbf{k},j} \tau_{\mathbf{k}}$, the conductivity takes the form

$$\sigma_{ij} = X_{ij}(E_F) = e^2 \langle v_{\mathbf{k},i} v_{\mathbf{k},j} \tau_{\mathbf{k}} \rangle_{E_F} g(E_F). \tag{7}$$

Under the assumption of statistical independence between velocity components and relaxation times on the Fermi surface, that is, $\langle v_{\mathbf{k},i} v_{\mathbf{k},j} \tau_{\mathbf{k}} \rangle_{E_F} = \langle v_{\mathbf{k},i} v_{\mathbf{k},j} \rangle_{E_F} \langle \tau_{\mathbf{k}} \rangle_{E_F}$ [4], and for an isotropic system where $\sigma_{11} = \sigma_{22} = \sigma_{33}$, the velocity average simplifies to

$$\langle v_{\mathbf{k},i} v_{\mathbf{k},j} \rangle_{E_F} = \frac{1}{3} \delta_{ij} \langle v_{\mathbf{k}}^2 \rangle_{E_F}. \tag{8}$$

Thus, the zero-temperature conductivity, or equivalently the inverse residual resistivity, is given by

$$\sigma = \frac{e^2}{3} \langle v_{\mathbf{k}}^2 \rangle_{E_F} \langle \tau_{\mathbf{k}} \rangle_{E_F} g(E_F). \tag{9}$$

This semiclassical treatment implies that in isotropic systems, the residual resistivity follows an inverse proportionality, $\rho \propto g(E_F)^{-1}$ [5].

Alternatively, by integrating over the Fermi surface rather than performing a direct integration in the $\mathbf{k}$-space, and again assuming statistical independence of velocity and lifetime, the conductivity can be expressed as [4]

$$\sigma = \frac{e^2}{12\pi^3 \hbar} \lambda \mathcal{A}. \tag{10}$$

Here, the mean free path of the electron is given by $\lambda = \langle v_{\mathbf{k}} \rangle_{E_F} \langle \tau_{\mathbf{k}} \rangle_{E_F}$, and the total Fermi surface area satisfies $\int dS = 2\mathcal{A}$. The mean free path can also be obtained from the Fermi surface average of the electronic coherence length, defined as $\lambda = \langle \xi_{\mathbf{k}F} \rangle E_F$ [4], where

$$\xi_{\mathbf{k}F} = \pi \int_{-\infty}^{E_F} \mathrm{d}E \frac{\partial A_{\mathbf{k},E}}{\partial k}. \tag{11}$$

Here, $A_{\mathbf{k},E}$ denotes the Bloch spectral function (BSF), which may be thought as $\mathbf{k}$ resolved density of states or band structure. Thus, the conductivity is also governed by the $\mathbf{k}$-space broadening of the band structure, with increased smearing leading to reduced conductivity.

Fig. 3 presents the site and band-resolved density of states at the Fermi level, $g(E_F)$, for AlTiVNb, where the contributions from delocalized *sp* electrons are shown as solid lines and those from localized *df* orbitals as dashed lines. (Contributions from $f$ states, *i.e.* $l = 3$, make a near-negligible contribution in the considered systems.) The 1a sublattice is represented in blue, while the 1b sublattice is represented in orange. With increasing order parameter $\eta$, the *df* DoS at $E_F$ decreases significantly for the 1a site, whereas the corresponding *sp* DoS exhibits a comparatively weaker reduction. In contrast, for the 1b site, the *sp* DoS shows a more pronounced decrease, while the *df* DoS increases.

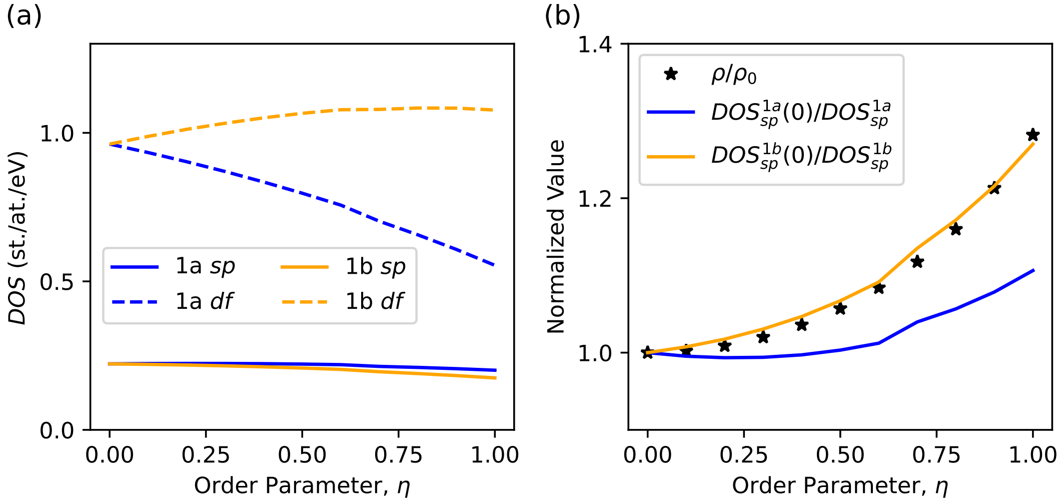


FIG. 3. (a) Comparison of the site- and band-resolved density of states (DoS) at the Fermi level $g(E_F)$ for AlTiVNb as a function of increasing order parameter $\eta$. Solid lines correspond to contributions from delocalized *sp* electrons, while dashed lines represent localized *df* states. The 1a sublattice is shown in blue, and the 1b sublattice in orange. (b) Comparison of the computed resistivity ratio from the *SPR-KKR* Kubo formalism (black filled stars) and the site-resolved relative changes in the *sp* DoS for AlTiVNb as a function of increasing order parameter $\eta$. The solid blue and orange lines correspond to the 1a and 1b sublattices, respectively.

Focusing on mobile charge carriers, which are mainly associated with the *sp* bands, the relative change in resistivity can be estimated using $\rho \propto g(E_F)^{-1}$, under the assumption that the scattering properties encoded in $\langle v_{\mathbf{k}}^2 \rangle_{E_F} \langle \tau_{\mathbf{k}} \rangle_{E_F}$ remain unchanged with increasing $\eta$. The resistivity ratio is thus given by

$$\frac{\rho(\eta)}{\rho_0(\eta = 0)} = \frac{g_{\rm sp}(E_F, \eta = 0)}{g_{\rm sp}(E_F, \eta)}. \tag{12}$$

Fig. 3(b) compares the computed resistivity ratio from the *SPR-KKR* Kubo formalism (black filled stars) with the site-resolved relative changes in the *sp* DoS, where the solid blue and orange lines correspond to the 1a and 1b sublattices, respectively. A near perfect agreement is observed, which confirms that the increase in residual resistivity with increasing $\eta$ is mainly associated with the reduction of the *sp* DoS at the 1a site. Although the *sp* DoS at the 1b site also decreases, its effect on the overall resistivity is less pronounced. Both sites contribute to the total conductivity, suggesting that additional scattering effects, particularly at the 1b site, where only three elements remain (excluding Al), may play a role in further increasing the resistivity, assuming equal contributions from both sites.

For AlTiCrMo, a similar trend is observed, but the dominant changes occur in the 1b sublattice (solid blue line in Fig. 4(b)), while the 1a site exhibits a weaker increase in the $g_{\rm sp}(E_F, \eta = 0)/g_{\rm sp}(E_F, \eta)$ ratio. These findings strongly indicate that, in both AlTiVNb and AlTiCrMo, the increase in resistivity with increasing $\eta$ is directly correlated with the depletion of *sp* DoS at the Fermi level, which is induced by Al expressing a strong sublattice preferencein the B2 ordered structures for both alloys.

The top panels of Figs. 5 and 6 then depict the BSF along high-symmetry directions for the B2 structure in AlTiVNb RSA, with increasing values of $\eta = 0.0, 0.5, 1.0$. Then the bottom panels depict the corresponding constant-energy cut planes ($E = E_F$) of the BSF along $\mathbf{k}_x$ [100] and $\mathbf{k}_y$ [010] through the $\Gamma$-point at $\mathbf{k}_z = (0, 0, 0)$, with the respective high-symmetry points indicated. The trends observed in the DoS analysis are directly reflected in the BSF intensity.

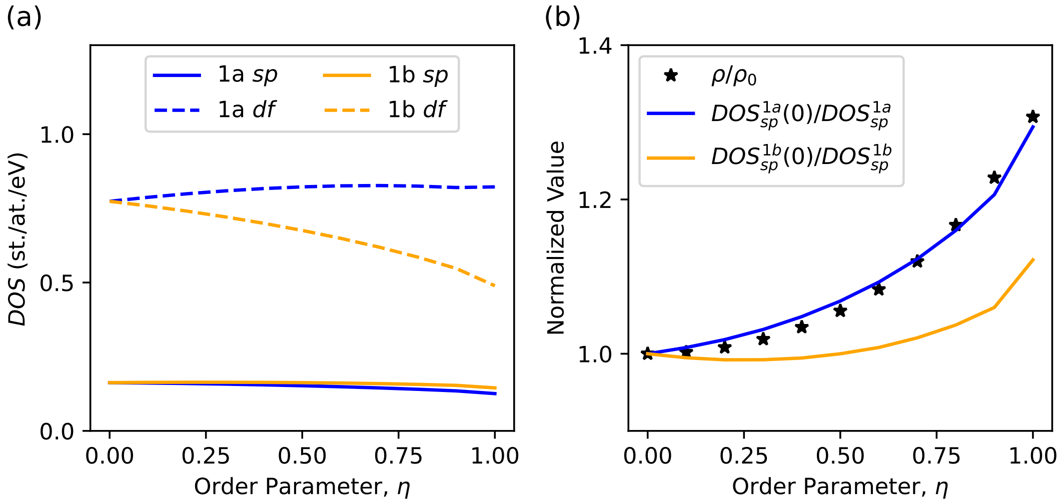


FIG. 4. (a) Comparison of the site- and band-resolved density of states (DoS) at the Fermi level $g(E_F)$ for AlTiCrMo RSA as a function of increasing order parameter $\eta$. Solid lines correspond to contributions from delocalized *sp* electrons, while dashed lines represent localized *df* states. The 1a sublattice is shown in blue, and the 1b sublattice in orange. (b) Comparison of the computed resistivity ratio from the *SPR-KKR* Kubo formalism (black filled stars) and the site-resolved relative changes in the *sp* DoS for AlTiCrMo RSA as a function of increasing order parameter $\eta$. The solid blue and orange lines correspond to the 1a and 1b sublattices, respectively.

The depletion of *df* states at the Fermi edge for the 1a site is clearly visible along the high-symmetry $\mathbf{k}$ path and in the cut $\mathbf{k}_x\mathbf{k}_y$. In contrast, for the 1b site, the *df* DoS at the Fermi level increases with increasing $\eta$, which is directly evident from the enhanced BSF intensity.

This behaviour is particularly pronounced along the $\Gamma - M$ and $\Gamma - X - M$ directions, where the contrast between the low-intensity pocket at the $M$ point and the states at other high-symmetry points is evident. However, direct extraction of $k$-space smearing, and consequently the electron mean free path, is nontrivial from this representation. Based on the BTE results, enhanced $k$-space broadening effects are expected predominantly for the 1a site in AlTiVNb. Examination of the BSF cuts, where additional thin white lines indicate isointensity contours, suggests that these contours are more widely spaced for the 1a site compared to the 1b site, thus increasing $\delta\mathbf{k}$ for a constant $\Delta A_{\mathbf{k},E}$. However, this observation should be interpreted with caution, as this visualization does not correspond to a rigorous evaluation of Eq. 11.

For AlTiCrMo, the BSF along high-symmetry directions in reciprocal space is shown in the top panels of Fig. 7 for the 1a site and in Fig. 8 for the 1b site, with the corresponding constant energy cut planes ($E = E_F$) along $\mathbf{k}_x$ [100] and $\mathbf{k}_y$ [010] presented in the lower panels. The evolution of the electronic structure is more complex as the sublattices exhibit distinct redistribution patterns. For example, in the 1a sublattice, the states initially localized at the $X$-point for $\eta = 0$ are gradually shifted towards the $M$-point with increasing $\eta$, leading to the formation of a pocket at the $\Gamma$ point. A detailed analysis of these effects is more intricate, and a direct assessment of $k$-space smearing would require explicit determination of $n(\mathbf{k})$ from the BSF, which is beyond the scope of the present study.

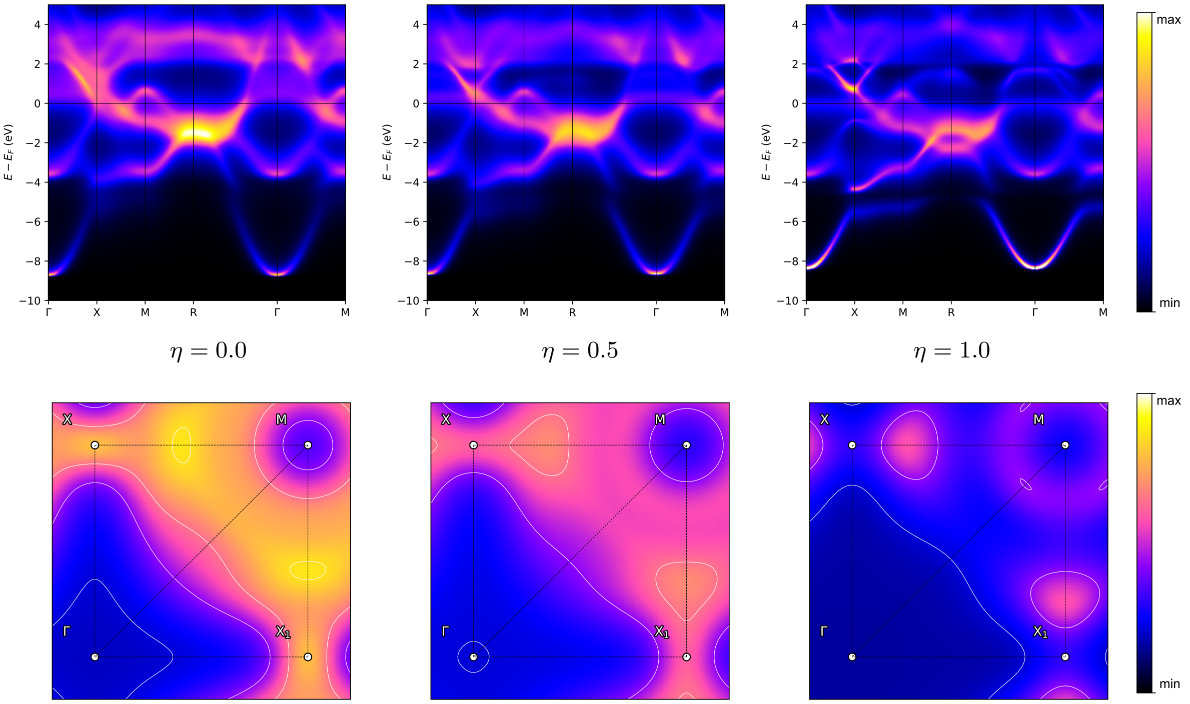


FIG. 5. Plots of the Bloch spectral function (BSF) along high-symmetry directions for the AlTiVNb RSA resolved into its contribution from the 1a site within the bcc B2 structure for increasing order parameter $\eta = 0.0, 0.5, 1.0$. The corresponding energy cut planes of the BSF at the Fermi level along $\mathbf{k}_x$ [100] and $\mathbf{k}_y$ [010] through the Γ-point at $\mathbf{k}_z = (0, 0, 0)$ are shown below, with high-symmetry points indicated.

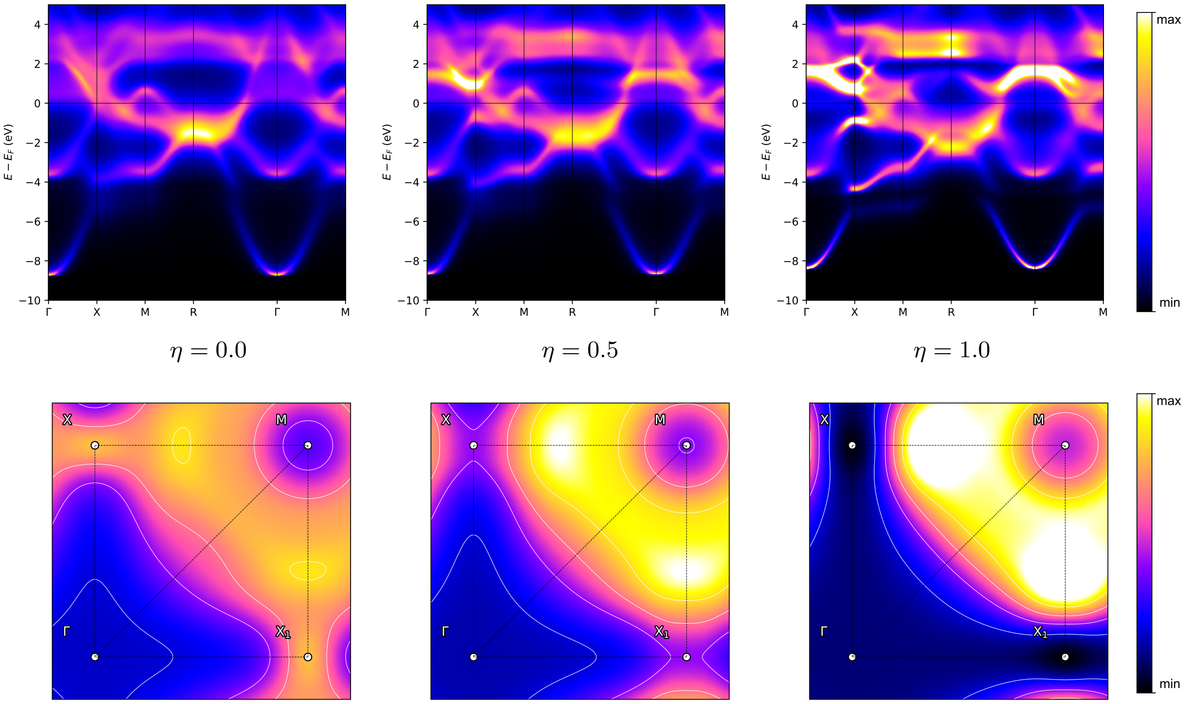


FIG. 6. As Fig. 5 but for the 1b site.

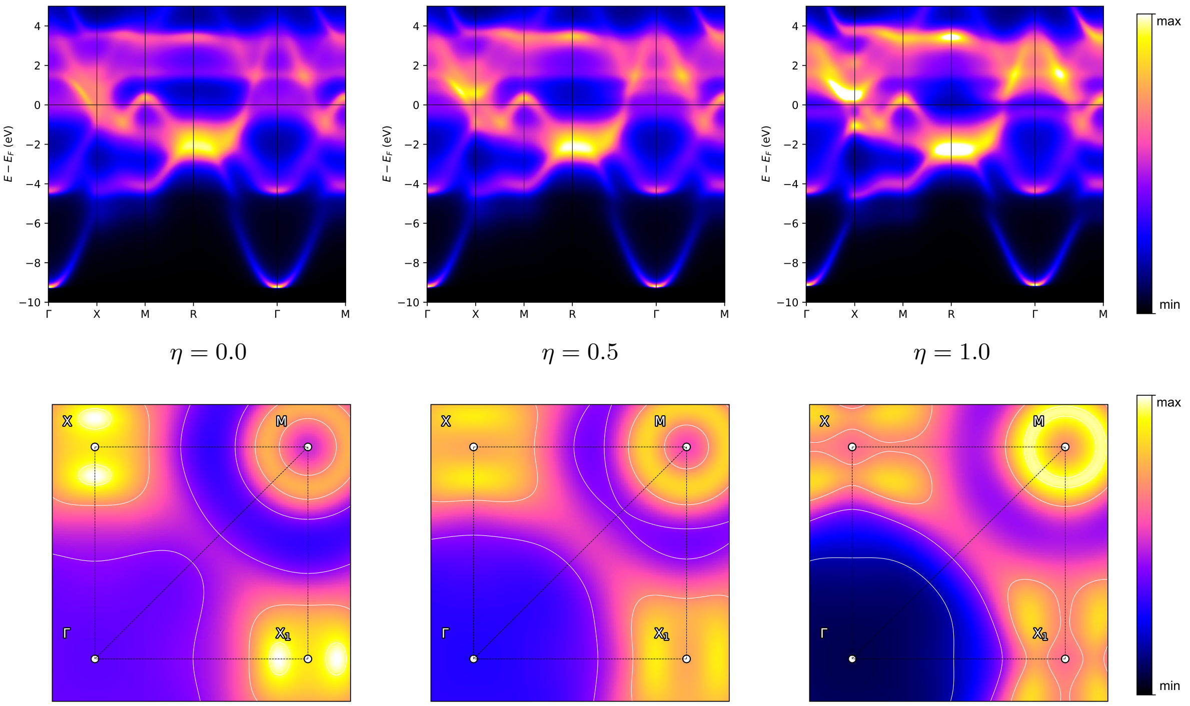


FIG. 7. Plots of the Bloch spectral function (BSF) along high-symmetry directions for the AlTiCrMo RSA resolved into its contribution from the 1a site within the bcc B2 structure for increasing order parameter $\eta = 0.0, 0.5, 1.0$. The corresponding energy cut planes of the BSF at the Fermi level along $\mathbf{k}_x$ [100] and $\mathbf{k}_y$ [010] through the Γ-point at $\mathbf{k}_z = (0, 0, 0)$ are shown below, with high-symmetry points indicated.

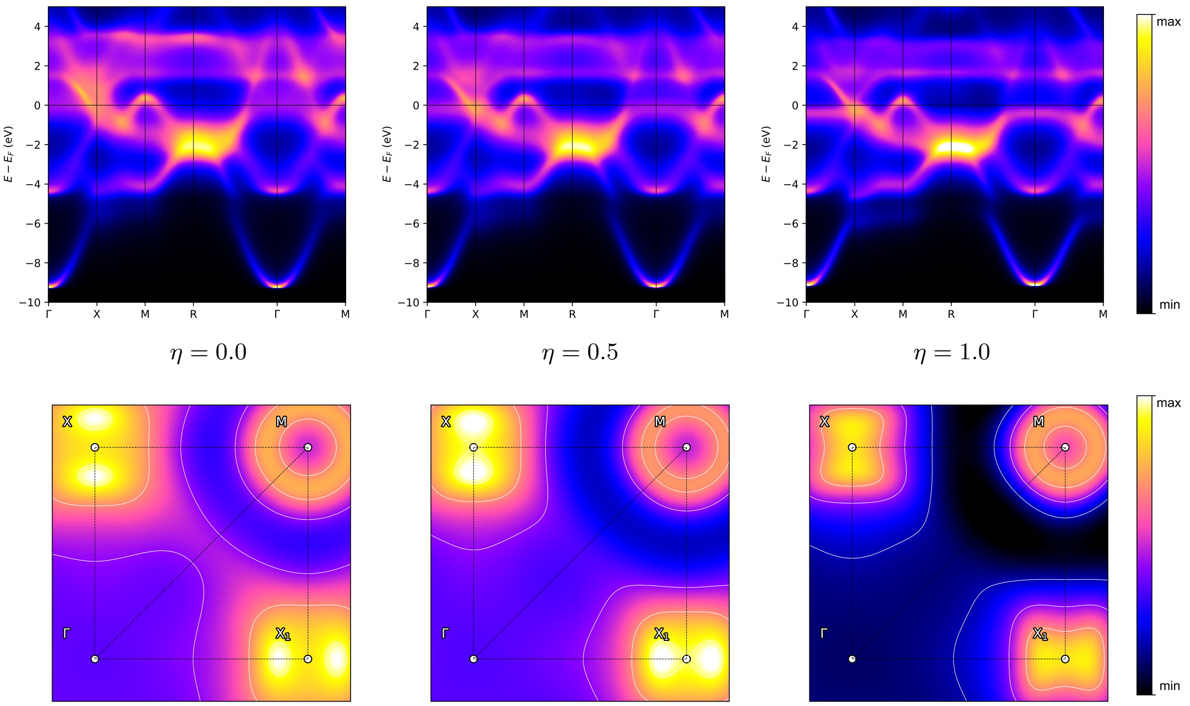


FIG. 8. As Fig. 7 but for the 1b site.

[1] J. M. Ziman, *Principles of the Theory of Solids*, 2nd ed. (Cambridge University Press, 1972).
[2] G. D. Mahan and J. O. Sofo, Proceedings of the National Academy of Sciences **93**, 7436 (1996).
[3] T. J. Scheidemantel, C. Ambrosch-Draxl, T. Thonhauser, J. V. Badding, and J. O. Sofo, Physical Review B **68**, 125210 (2003).
[4] H. C. Robarts, T. E. Millichamp, D. A. Lagos, J. Laverock, D. Billington, J. A. Duffy, D. O'Neill, S. R. Giblin, J. W. Taylor, G. Kontrym-Sznajd, M. Samsel-Czekała, H. Bei, S. Mu, G. D. Samolyuk, G. M. Stocks, and S. B. Dugdale, Physical Review Letters **124**, 046402 (2020).
[5] G. D. Samolyuk, S. Mu, A. F. May, B. C. Sales, S. Wimmer, S. Mankovsky, H. Ebert, and G. M. Stocks, Physical Review B **98**, 165141 (2018).
